# Supplementary material for: DataScribe: An AI-Native, Policy-Aligned Web Platform for Multi-Objective Materials Design and Discovery
Source: arXiv:2601.07966 source file (2026-01-12)
Supplement: Supplementary file 1 [file 13_appendix.tex]

\appendix
\section{XGBoost Regression with \emph{datascribe\_api}} \label{app:datascribe_xgboost}

The example Python script below shows how to retrieve a data table from the \emph{datascribe\_api}~\cite{datascribe_api_2025}, prepare it for regression, and train an XGBoost model to predict the Creep Merit property from selected alloying elements. Model performance is assessed using standard error metrics, and a parity plot is generated to visualize the agreement between predicted and actual values.

\begin{tcolorbox}[breakable, colback=gray!10,colframe=gray!50,title=\emph{datascribe\_api} XGBoost Regression Example]
\begin{minted}{python}
"""Train an XGBoost regressor on DataScribe data and visualize performance."""

import matplotlib.pyplot as plt
import pandas as pd
from sklearn.metrics import mean_absolute_error, r2_score, root_mean_squared_error
from sklearn.model_selection import train_test_split
from xgboost import XGBRegressor

from datascribe_api import DataScribeClient

TABLE_NAME = "iqr_dataframe"
COLUMNS = ["Nb", "Cr", "V", "W", "Zr", "Creep_Merit"]
TARGET_COL = "Creep_Merit"

with DataScribeClient() as client:
    df = client.get_data_table_rows(
            tableName=TABLE_NAME,
            columns=COLUMNS,
            numRows=1000
    ).to_dataframe()

X, y = df.drop(columns=TARGET_COL), df[TARGET_COL]

X_train, X_test, y_train, y_test = train_test_split(
    X, y, test_size=0.25, random_state=18
)

xgb = XGBRegressor(
    n_estimators=600,
    learning_rate=0.02,
    max_depth=8,
    subsample=0.8,
    colsample_bytree=0.8,
    reg_lambda=1.0,
    random_state=84,
    n_jobs=-1,
    tree_method="hist",
    eval_metric="rmse",
)

xgb.fit(X_train, y_train, verbose=False)
y_pred = xgb.predict(X_test)

metrics = {
    "R2": r2_score(y_test, y_pred),
    "MAE": mean_absolute_error(y_test, y_pred),
    "RMSE": root_mean_squared_error(y_test, y_pred),
}

fig, ax = plt.subplots(figsize=(5, 5))

ax.scatter(y_test, y_pred, alpha=0.6)
lims = [min(y_test.min(), y_pred.min()), max(y_test.max(), y_pred.max())]
ax.plot(lims, lims, "k--", lw=2, label="Perfect prediction")

ax.set_xlabel("Actual Creep Merit")
ax.set_ylabel("Predicted Creep Merit")
ax.set_xscale("log")
ax.set_yscale("log")
ax.set_title(
    f"XGBoost Parity Plot\n"
    f"R²={metrics['R2']:.3f}, RMSE={metrics['RMSE']:.3f}"
)
ax.legend()
plt.show()
\end{minted}
\end{tcolorbox}
